# Supplementary material for: On the Generalization Capability of Temporal Graph Learning Algorithms: Theoretical Insights and a Simpler Method
Source: arXiv:2402.16387 source file (2024-02-26)
Supplement: Supplementary file 1 [file feature-label-alignment.tex]

In this section, we provide insights on why feature-label alignment (FLA) is important by reviewing how this term appears in the convergence and generalization of existing works.

\subsection{Feature label alignment in \cite{arora2019fine}}

\cite{arora2019fine} shows that for any 1-Lipschitz loss function the generalization error of the two-layer infinite-wide ReLU network found by GD is bounded by the feature-label alignment term \begin{equation*}
    \sqrt{\frac{\mathbf{y}^\top (\mathbf{H}^\infty)^{-1} \mathbf{y}}{N}},
\end{equation*}
where $\mathbf{H}^\infty$ is the neural tangent kernel of infinite-wide two-layer ReLU network.
Our results in Theorem~\ref{theorem:all_generalization} is similar to their results, however, our results hold for multi-layer neural network with different activation functions (e.g., ReLU, LeakyReLU, Sigmoid, and Tanh) without the infinite-wide assumption.

\subsection{Feature label alignment in~\cite{}}
For any positive definite matrix $\mathbf{K} \in \mathbb{R}^{N\times N}$, we have
\begin{equation*}
    \frac{1}{\lambda_{\min}(\mathbf{K})} = \lambda_{\max}(\mathbf{K}^{-1}) = \max_{\mathbf{y} \in \mathbb{R}^N} \frac{\mathbf{y}^\top (\mathbf{K}^{-1}) \mathbf{y}}{\| \mathbf{y} \|_2^2}
\end{equation*}
which implies the following equality \begin{equation*}
    \mathbf{y}^\top (\mathbf{K}^{-1}) \mathbf{y} \leq \frac{\| \mathbf{y} \|_2^2}{\lambda_{\min}(\mathbf{K})}
\end{equation*}
In other word, the feature-label alignment is proportional to $1/\lambda_{\min}(\mathbf{K})$. In the following, we show the connection between $1/\lambda_{\min}(\mathbf{K})$ to the convergence speed of neural network in the theoretical analysis.
