# Supplementary material for: On the Generalization Capability of Temporal Graph Learning Algorithms: Theoretical Insights and a Simpler Method
Source: arXiv:2402.16387 source file (2024-02-26)
Supplement: Supplementary file 2 [file lower_bound_eigenvalue_ffn.tex]

\section{Lower bound on FFN}

Consider an $L$-layer ReLU network
\begin{equation*}
    \mathbf{h}^{(\ell)}_i = \begin{cases}
    \mathbf{x}_i & \text{ if } \ell=0 \\
    \sigma(\mathbf{h}^{(\ell-1)}_i \mathbf{W}^{(\ell)}) & \text{ if } \ell\in\{ 1,\ldots,L-1 \}\\
    \mathbf{h}^{(L-1)}_i \mathbf{W}^{(L)} & \text{ if } \ell=L 
    \end{cases}
\end{equation*}
where $\mathbf{W}^{(\ell)} \in \mathbb{R}^{d_{\ell-1} \times d_\ell}$. We assume the network has a single output with $d_L = 1$. We denote $\mathbf{z}^{(\ell)}$ as the pre-activation that $\mathbf{h}^{(\ell)} = \sigma(\mathbf{z}^{(\ell)})$.

Let us define $\bm{\theta} = [\text{vec}(\mathbf{W}^{(1)}),\ldots,\text{vec}(\mathbf{W}^{(L)})]$ and $\mathbf{H}_\ell(\bm{\theta}) = [\mathbf{h}_1^{(\ell)}, \ldots, \mathbf{h}_N^{(\ell)}]$. For notation simplicity, we can omit the term in the parenthesis.

Let $\mathbf{J}$ be the Jacobian of 
\begin{equation*}
    \mathbf{J} = \left[ \frac{\partial \mathbf{H}_L}{\partial \text{vec}(\mathbf{W}^{(1)})}, \ldots, \frac{\partial \mathbf{H}_L}{\partial \text{vec}(\mathbf{W}^{(L)})}\right] \in \mathbb{R}^{N \times \sum_{\ell=1}^L d_{\ell-1} d_\ell}
\end{equation*}

The empirical NTK Gram matrix denoted by 
\begin{equation}
    \Bar{\mathbf{K}}^{(L)} = \mathbf{J} \mathbf{J}^\top = \sum_{\ell=1}^L \left[ \frac{\partial \mathbf{H}_L}{\partial \text{vec}(\mathbf{W}^{(\ell)})} \right] \left[ \frac{\partial \mathbf{H}_L}{\partial \text{vec}(\mathbf{W}^{(\ell)})} \right]^\top
\end{equation}

We denote $\mathbf{\Sigma}^\ell_i = \text{diag}([\sigma^\prime(z_{ij}^{(\ell)})]_{j=1}^{d_\ell}) \in \mathbb{R}^{d_\ell \times d_\ell}$.

By the chain rules, we know that 
\begin{equation*}
    \begin{aligned}
    \mathbf{J} \mathbf{J}^\top 
    &= \sum_{\ell=1}^L \left[ \frac{\partial \mathbf{H}_L}{\partial \text{vec}(\mathbf{W}^{(\ell)})} \right] \left[ \frac{\partial \mathbf{H}_L}{\partial \text{vec}(\mathbf{W}^{(\ell)})} \right]^\top \\
    &= \sum_{\ell=1}^{L} \mathbf{H}_{\ell-1} \mathbf{H}_{\ell-1}^\top \odot \mathbf{B}_\ell \mathbf{B}_\ell^\top
    \end{aligned}
\end{equation*}
where $\mathbf{B}_\ell \in \mathbb{R}^{N \times d_\ell}$ is a matrix whose $i$th row is given by
\begin{equation*}
    [\mathbf{B}_\ell]_{i,:} = \begin{cases}
    \mathbf{\Sigma}_i^\ell \left( \prod_{k=\ell+1}^{L-1} \mathbf{W}^{(\ell)} \mathbf{\Sigma}^\ell_i\right) \mathbf{W}_L & \text{ if } \ell\in \{1,\ldots,L-2\} \\
    \mathbf{\Sigma}_i^{L-1} \mathbf{W}_L & \text{ if } \ell= L-1\\
    1 & \text{ if } \ell = L 
    \end{cases}
\end{equation*}

For PSD matrices $\mathbf{P}, \mathbf{Q} \in \mathbb{R}^{d\times d}$, it holds $\lambda_{\min}(\mathbf{P} \odot \mathbf{Q}) \geq \lambda_{\min}(\mathbf{P}) \cdot \min_{i\in [d]} Q_ii $.

Thus, we know $\lambda_{\min}(\mathbf{J} \mathbf{J}^\top )$ has the following inequality holds
\begin{equation*}
    \lambda_{\min}(\mathbf{J} \mathbf{J}^\top ) = \sum_{\ell=1}^{L} \mathbf{H}_{\ell-1} \mathbf{H}_{\ell-1}^\top \odot \mathbf{B}_\ell \mathbf{B}_\ell^\top \geq \sum_{\ell=1}^{L} \lambda_{\min}( \mathbf{H}_{\ell-1} \mathbf{H}_{\ell-1}^\top) \cdot \min_{d\in[N]} \| [\mathbf{B}_\ell]_{i,:} \|_2^2
\end{equation*}
